# Supplementary material for: Rotational symmetry breaking in the topological superconductor Sr$_x$Bi$_2$Se$_3$ probed by upper-critical field experiments
Source: arXiv:1603.04197 source file (2016-03-14)
Supplement: Supplementary file 1 [file Supplementary_Information_Pan.pdf]

**SUPPLEMENTARY INFORMATION**

# Rotational symmetry breaking in the topological superconductor $Sr_xBi_2Se_3$ probed by upper-critical field experiments

Y. Pan[1], A. M. Nikitin[1], G. K. Araizi[1], Y. K. Huang[1], Y. Matsushita[2], T. Naka[2] and A. de Visser[1]

[1]*Van der Waals - Zeeman Institute, University of Amsterdam, Science Park 904, 1098 XH Amsterdam, The Netherlands*
[2]*National Institute for Materials Science, Sengen 1-2-1, Tsukuba, Ibaraki 305-0047, Japan*

## 1. Powder X-ray diffraction

Powder X-ray diffraction patterns have been obtained for $Sr_{0.10}Bi_2Se_3$ and $Sr_{0.15}Bi_2Se_3$. The patterns are in excellent agreement with the calculated pattern for $Bi_2Se_3$ and the $R\bar{3}m$ space group (see Fig. S1). The lattice parameters ($a$ = 4.137 Å and $c$ = 28.65 Å) are identical for both compositions within the experimental resolution. The tiny extra peaks (black arrows) in the diffraction pattern of $Sr_{0.15}Bi_2Se_3$ points to the presence of a minority impurity phase.

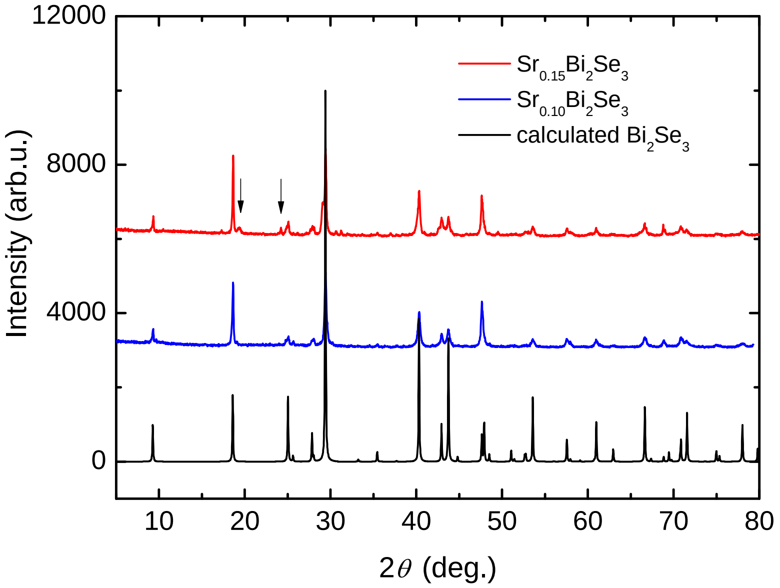


Fig. S1 *Powder X-ray diffraction pattern of $Sr_{0.10}Bi_2Se_3$ (blue line) and $Sr_{0.15}Bi_2Se_3$ (red line) at room temperature. The black line is the calculated pattern for $Bi_2Se_3$.*

In order to investigate whether $Sr_{0.15}Bi_2Se_3$ undergoes a structural transition the powder X-ray diffraction pattern was measured down to $T$ = 10 K. No change in crystal structure was observed (see Fig. S2). The lattice parameters $a$ and $c$ both show a small decrease with decreasing temperature. The tiny extra peaks (black arrows) in the diffraction pattern point to the presence of a minority impurity phase.

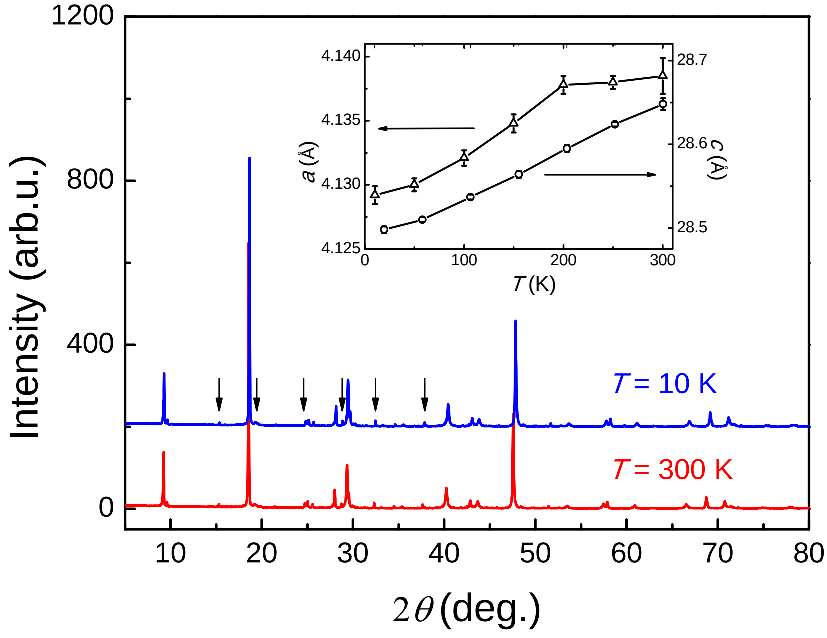


Fig. S2 *Powder X-ray diffraction pattern of* $Sr_{0.15}Bi_2Se_3$ *at 300 K (red line) and at 10 K (blue line). The inset shows the temperature variation of the lattice parameters a and c.*

## 2. Single-crystal Laue diffraction

Laue diffraction was made on the $Sr_xBi_2Se_3$ crystals to confirm their single-crystalline nature. The Laue diagrams show well defined spots and confirm the trigonal symmetry in the basal plane (see Fig. S3).

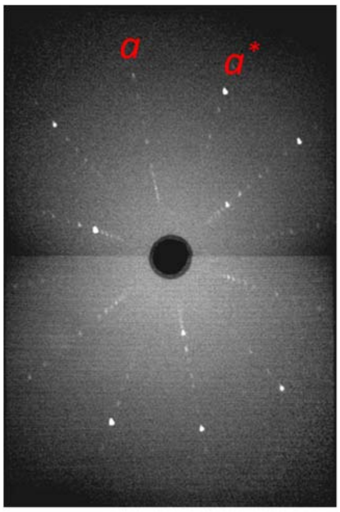


Fig. S3 *Back-scattering Laue diagram of $Sr_{0.15}Bi_2Se_3$ with the incoming beam along the c-axis. The diffraction pattern has trigonal symmetry. The a and a* axis are indicated.*

## 3. Sample shape and demagnetization factor

The basal-plane transport experiments were performed on thin-bar shaped samples with the current along the long axis. The sizes of the $Sr_{0.10}Bi_2Se_3$ crystal are 1.3×5.5×0.32 mm$^3$ and of the $Sr_{0.15}Bi_2Se_3$ crystal 1.3×2.3×0.35 mm$^3$. We have estimated the demagnetization factor *N* for the field along and perpendicular to the long axis (see Chen *et al.*, IEEE Transactions on Magnetics **38** (2002) 1742). For $Sr_{0.10}Bi_2Se_3$ we estimate $N_{\|} = 0.05$ and $N_{\perp} = 0.213$, and for $Sr_{0.15}Bi_2Se_3$ $N_{\|} = 0.12$ and $N_{\perp} = 0.20$. For a Type II superconductor a demagnetization factor $N \neq 0$ gives rise to a correction of the internal field $H_{in} = (B_{app}/\mu_0)/(1+ \chi N)$. We conclude these corrections are relatively small for our crystals and we neglect demagnetization effects. Neglecting the effect of *N* does not have a significant effect on the derived values of the large basal-plane anisotropy of the upper critical field $B_{c2}$.

## 4. Sample characterization: resistance and ac-susceptibility

The temperature variation of the resistivity, $\rho(T)$, of several $Sr_xBi_2Se_3$ crystals has been measured with a standard 4-probe low-frequency ac-technique in the PPMS. Typical resistivity traces, taken in the temperature range 2-300 K, are shown in Fig. S4. The resistance shows a metallic behavior. The $\rho(T)$-values at low temperature amount to 0.60 and 0.75 mΩcm for $x$ = 0.10 and 0.15, respectively, and are in good agreement with the values reported previously (Liu *et al.* JACS **137**, 10512 (2015), Shruti *et al.*, PRB **92**, 020506R (2015)). The superconducting transition temperatures as determined by the midpoints of the transitions are 2.84 K and 2.95 K for $x$ = 0.10 and 0.15, respectively. The ac-susceptibility, $\chi_{AC}$, was measured in a driving field of 0.026 mT in the 3-Helium cryostat for several crystals with different sizes. The $\chi_{AC}$ data yield superconducting volume fractions of 5-40 % for $x$ = 0.10 and 80 % for 0.15, respectively.

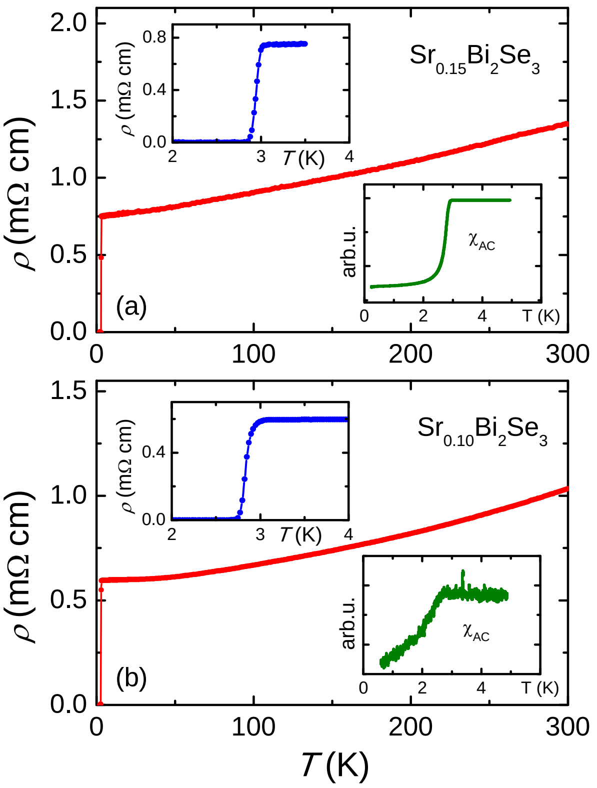


Fig. S4 *Panel (a) and (b): Resistivity of $Sr_xBi_2Se_3$ single crystals with $x$ = 0.15 and 0.10, respectively. Upper insets: zoom of the superconducting transition. Lower insets: ac-susceptibility around the superconducting transition.*

## 5. Superconducting transition in magnetic field of $Sr_{0.10}Bi_2Se_3$

The suppression of the superconducting state by a magnetic field was measured by the resistance as a function of temperature in fixed magnetic fields. The data for $Sr_{0.15}Bi_2Se_3$ taken in the PPMS down to a temperature of 2 K are shown in Fig. S5. The superconducting transition temperatures are determined by the midpoints of the transitions.

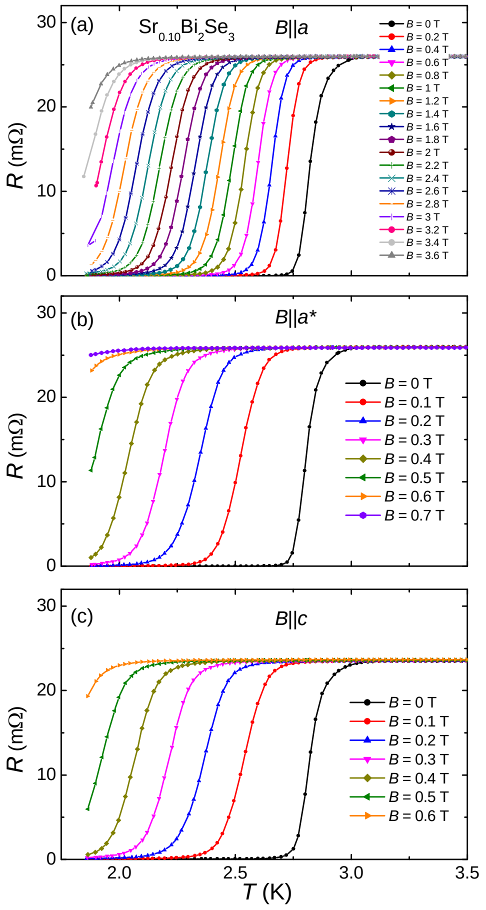


Fig. S5 *Superconducting transition of* $Sr_{0.10}Bi_2Se_3$ *measured in fixed magnetic fields as indicated. In panel (a), (b) and (c) the B-field is applied along the a, a* and c-axis, respectively.*

## 6. Superconducting transition in magnetic field of $Sr_{0.15}Bi_2Se_3$

The suppression of the superconducting state by a magnetic field was measured by the resistance as a function of temperature in fixed magnetic fields. The data for $Sr_{0.15}Bi_2Se_3$ taken in the 3-Helium cryostat down to 0.3 K are shown in Fig. S6. The superconducting transition temperatures are determined by the midpoints of the transitions. For $B \parallel a$ the resistance develops a small tail towards $R = 0$, which is attributed to a sample inhomogeneity.

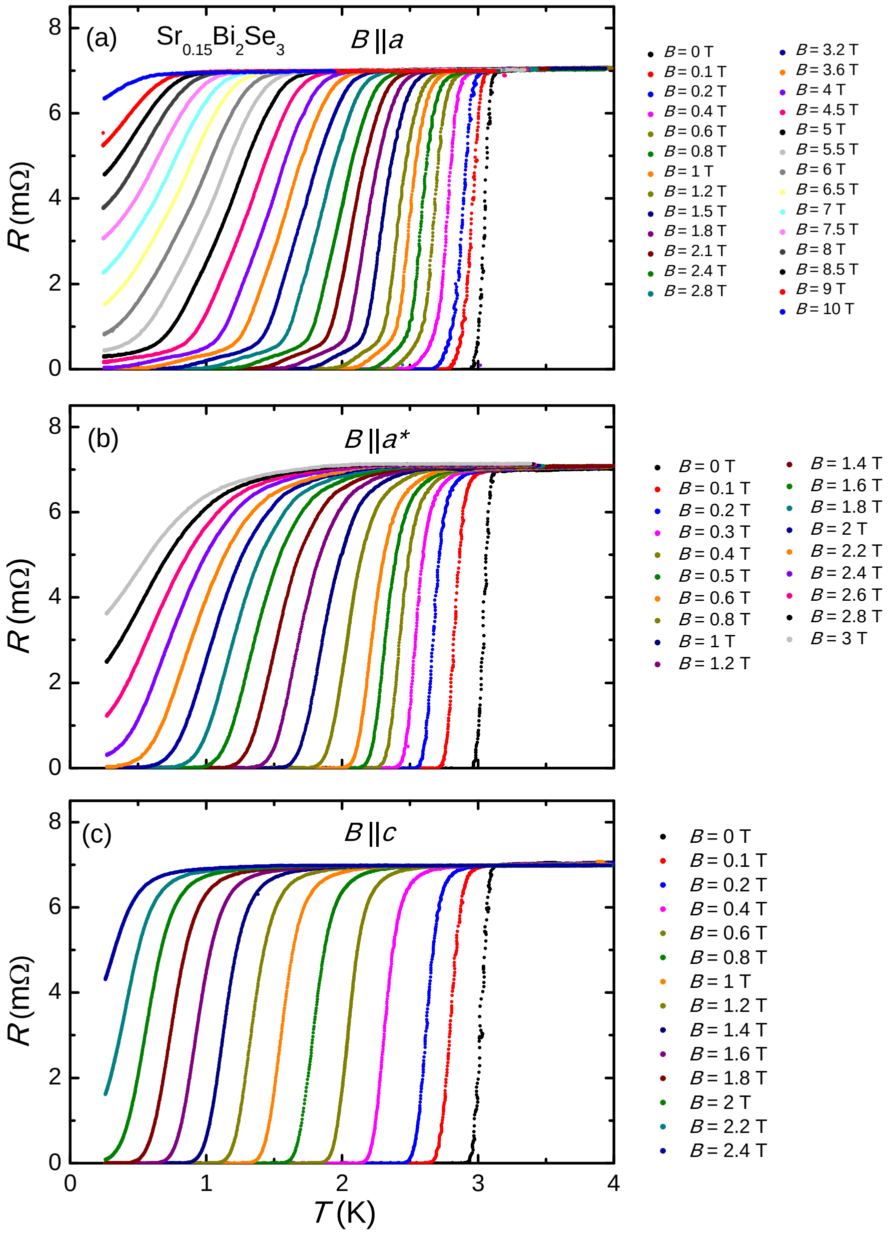


Fig. S6 *Superconducting transition of $Sr_{0.15}Bi_2Se_3$ measured in fixed magnetic fields as indicated. In panel (a), (b) and (c) the B-field is applied along the a, a* and c-axis, respectively.*

## 7. Angular variation of the resistance as a function of magnetic field

The angular variation of $R(B)$ of the $Sr_{0.10}Bi_2Se_3$ crystal was measured in the PPMS at $T$ = 2.0 K, whereas data for $Sr_{0.15}Bi_2Se_3$ were taken at $T$ = 2.0 K in the PPMS and at $T$ = 0.3 K in the 3-Helium cryostat. Selected $R(B)$ curves are shown in Fig. S7. The midpoints of the transitions to the normal state determine $T_c(B)$ and have been used to construct Fig. 3 in the manuscript.

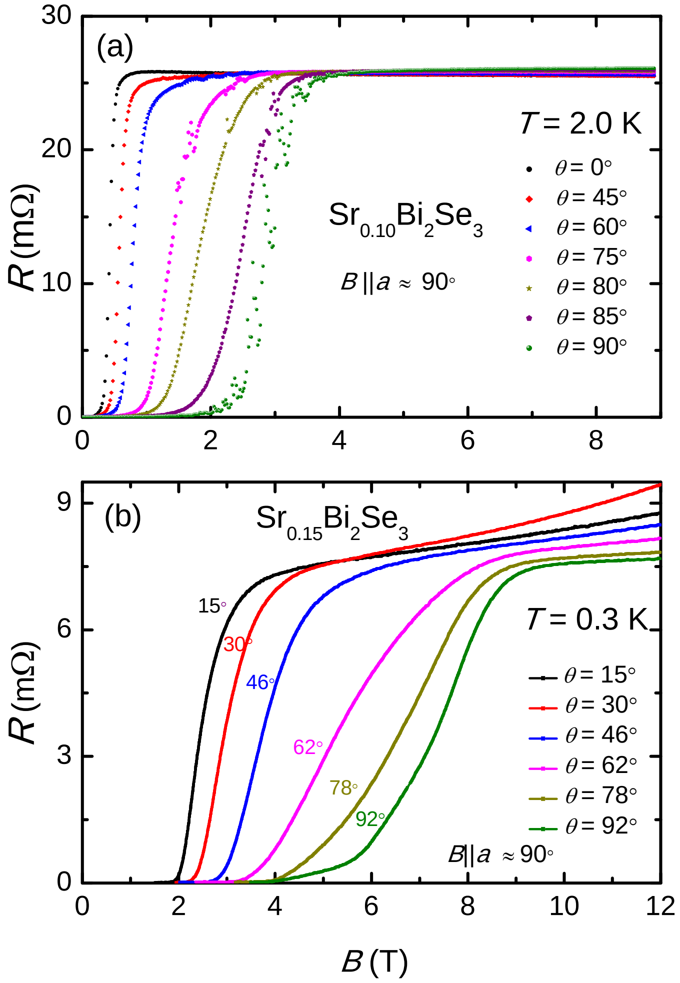


Fig. S7 *Panel (a) and (b): Angular variation of the magnetoresistance of* $Sr_{0.10}Bi_2Se_3$ *at 2.0 K and of* $Sr_{0.15}Bi_2Se_3$ *at 0.3 K, respectively. The angle* $\theta = 0°$ *corresponds to* $B \perp I$*. The angle* $\theta = 90°$ *corresponds to* $B \parallel I$*, which is also close to* $B \parallel a$*.*

## 8. Specific heat

The specific heat of a $Sr_{0.15}Bi_2Se_3$ crystal with mass 7.6 mg was measured by the relaxation method using the Heat Capacity Option in the PPMS in the temperature range 2-300 K. In Fig. S8 the data from 2 to 200 K are shown. No sign of a structural transition is found in this temperature range. The data between 200 and 300 K (not shown) show some irregularities that can be attributed to the Apiezon N grease that was used to fix the sample to the specific heat platform (see Heat Capacity Option Manual PPMS 2014, Part Number 1085-150 M5, Quantum Design).

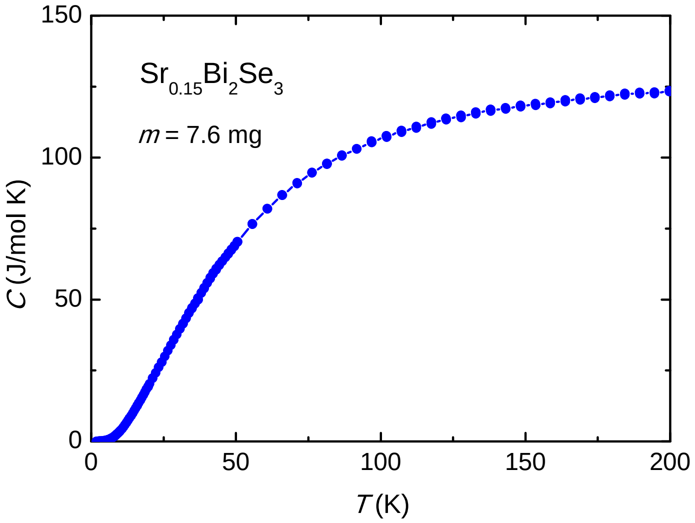


Fig. S8 *Specific heat of* $Sr_{0.15}Bi_2Se_3$ *as a function of temperature.*

## 9. Current dependence of *R*(θ)

The angular variation *R*(θ) of the $Sr_{0.10}Bi_2Se_3$ crystal was investigated for currents ranging from 0.1 to 2 mA at *T* = 2 K and *B* = 1 T. No significant changes are observed for currents $I \leq 1$ mA as shown in Fig. S9. The small increase in resistance for the largest current *I* = 2 mA is attributed to Joule heating.

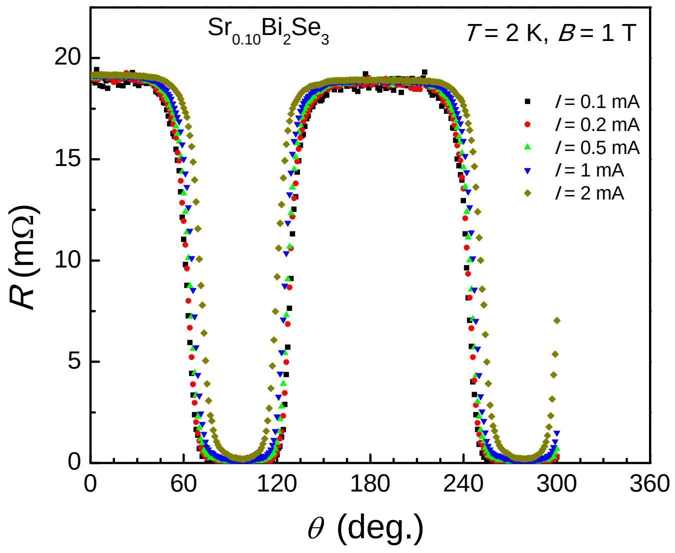


Fig. S9 *Angular variation R(θ) of* $Sr_{0.10}Bi_2Se_3$ *measured at T=2 K and B= 1 T for currents ranging from 0.1-2 mA as indicated.*

## 10. Transport measurements with the current along the *c*-axis

The angular variation $R(\theta)$ in the basal plane was measured with the current along the *c*-axis for $Sr_{0.15}Bi_2Se_3$. In this geometry the *B*-field is always perpendicular to the measuring current. Two circular gold electrodes (diameter 60 µm) were evaporated exactly opposite to each other on the basal-plane surfaces of a thin $Sr_{0.15}Bi_2Se_3$ single crystal (label #2) with dimensions 6×3×0.5 $mm^3$. Four copper wires (25 µm) that served as current and voltage leads were attached to the electrodes with silver paste, but effectively the resistance was measured in a two-point configuration. Data were taken in the PPMS in the temperature range 2-200 K with a current $I$ = 1 mA, see Fig. S10. Superconductivity results in a drop of 12% of the resistance. In this measurement configuration the transition is relatively broad, The onset temperature for superconductivity for this crystal is 2.75 K. The angular variation for $B$ = 0.5 T in the basal plane is shown in Fig. S11 in the $T$-range 2.0-3.5 K. The two-fold anisotropy is the same as in the measurements with the current in the basal plane for $x$ = 0.10 (Fig. 1 in the manuscript). For $B \perp I \parallel c$ the lowest resistance values and the largest values for $B_{c2}$ are found for the *B*-field along the long direction of the sample. After the measurements gold electrodes were evaporated at a different place opposite to each other on the basal plane surfaces and the experiment was repeated with essentially the same results and conclusions.

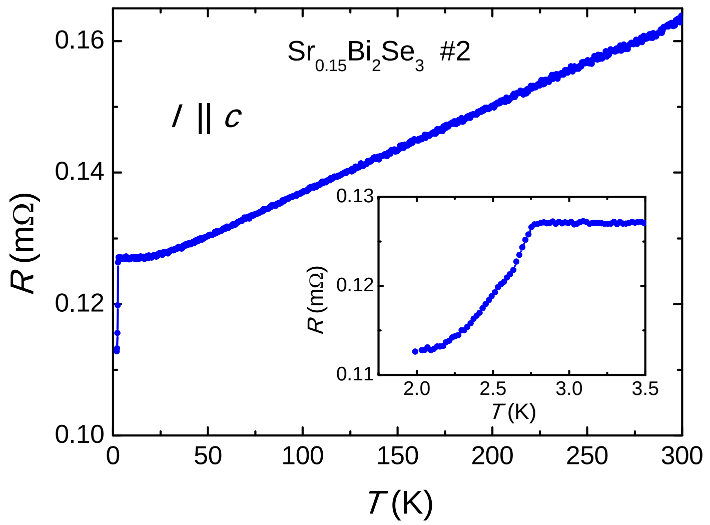


*Fig. S10 Resistance of $Sr_{0.15}Bi_2Se_3$ for I || c-axis, measured in a two-point configuration. Superconductivity results in a drop of 12% of the resistance. The residual resistance of 0.112 mΩ at 2.0 K is due to the silver paste and the copper wires.*

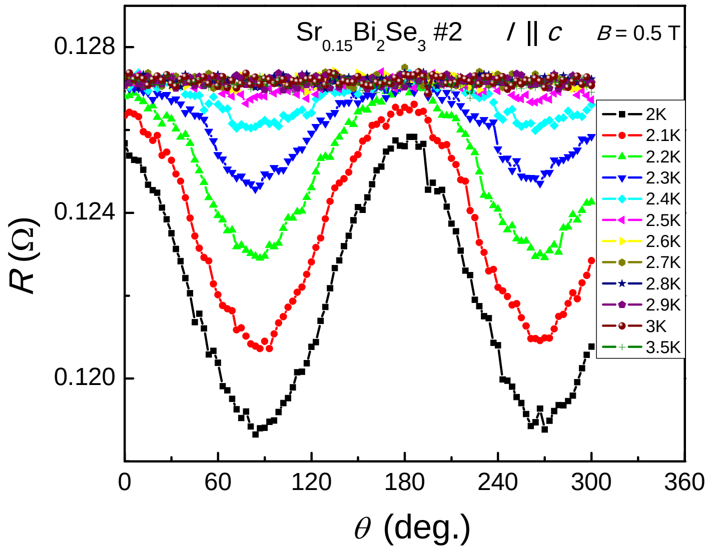


*Fig. S11 Angular variation R(θ) in the basal plane for I || c-axis for B = 0.5 T at temperatures as indicated. The lowest curve (black symbols) is at 2.0 K. The anisotropy is two-fold. The lowest resistance values and thus the largest values for $B_{c2}$ are found for the B-field along the long direction of the sample.*
